# Supplementary material for: Efficient NTK using Dimensionality Reduction
Source: arXiv:2210.04807 source file (2022-10-10)
Supplement: Supplementary file 1 [file appendix.tex]

\section{Appendix}
